# Supplementary material for: Anderson localization in an interacting fermionic system
Source: arXiv:1305.2018 ancillary file (2013-05-09)
Supplement: Supplementary file 1 [file Massel-Supp.pdf]

# Anderson localization in an interacting fermionic system-Supplementary Material I

Francesco Massel
*University of Helsinki, Department of Mathematics and Statistics, P.O. Box 68, FIN-00014, Finland*

## LOCALIZATION LENGTH

As pointed out in the main text, the localization length for in a non-interacting fermionic system in a lattice can be obtained following the description in terms of a classical Hamiltonian map proposed in [1]

$$\begin{aligned} l_{loc}^{-1}(V_0,\mu) &= \frac{1}{2}\int P(V)\ln\left(1+\frac{V^2}{4\sin^2\mu}\right)dV \\ &= \frac{1}{2}\ln\left[1+\frac{V_0^2}{16J^2\sin^2\mu}\right]+\frac{4\arctan\left[V_0/4J\sin\mu\right]}{V_0/J\sin\mu}-1, \end{aligned} \tag{1}$$

where

$$E = 2J\cos\mu \tag{2}$$

represents the energy eigenvalue for a single-particle state n presence of disorder. The largest value of $l_{loc}(V_0,\mu)$ is reached when $\sin\mu = 1$, implying that the largest value of the localization length is attained for $E = 0$, and therefore leading to the expression given in Eq. (2) for the global localization length of the non-interacting many-body system. In [1], it is pointed out that the expression given by Eq. (1), is valid in the range $V_0/J \sim 1-3$. In our simulations, however, we have found good agreement between the expression given by Eq. (2) of the main text and the numerical results up to $V_0/J \sim 5$.

## STRING HYPOTHESIS FOR THE LIEB-WU EQUATIONS

We show here how to gain some insight into the problem through the string hypothesis for the solution of the Lieb-Wu equations, whose solutions describe (most of) the eigenvalues of the Hubbard Hamiltonian in one dimension (Chapter 4 of [2]), in the limit of large lattice lengths $L$. For a fixed total number of particles $N$ and number of down particles $N_\downarrow$, the patterns of which the solutions of the Lieb-Wu equations are composed can be classified in three different categories:

- $k-\Lambda$ strings;
- single real values of $k_j$;
- $\Lambda$ strings.

Every eigenstate of the Hubbard Hamiltonian can be represented in terms of a particular configuration of strings, containing $M_n$ $\Lambda$-strings, $M'_n$ $k-\Lambda$ strings of length $n$, and $\mathcal{M}_e$ single $k_j$. Here $M_n$, $M'_n$, $\mathcal{M}_e$ are related to the $N$ and $N_\downarrow$ by

$$N_\downarrow = \sum_{n=1}^{\infty} n\left(M_n + M'_n\right) \tag{3}$$

$$N = \mathcal{M}_e + \sum_{n=1}^{\infty} 2nM'_n. \tag{4}$$

For $U$ sufficiently large ( $U > 8/L$, see [2]), the relevant solution for the spectrum of the Hubbard chain is characterized by

$$M'_1 = \frac{N}{2} - \mathcal{M}_e \tag{5}$$

$$M'_n = 0 \text{ for } n \neq 1. \tag{6}$$

In this case, the general expression for energy and momentum, given in terms of the relevant quantum numbers as

$$P = \left[ \sum_{j=1}^{N-2M'} k_j - \sum_{n=1}^{\infty} \sum_{\alpha=1}^{M'_n} \left( 2\,\mathrm{Re}\arcsin\left( {\Lambda'_\alpha}^n + niU/4J \right) - (n+1)\pi \right) \right] \mod 2\pi \tag{7}$$

$$E = -2J \sum_{j=1}^{N-2M'} \cos(k_j) + 4J \sum_{n=1}^{\infty} \sum_{\alpha=1}^{M'_n} \mathrm{Re}\sqrt{1 - \left(\Lambda'_\alpha + niU/4J\right)^2}. \tag{8}$$

assumes the following form

$$P = \sum_{j=1}^{N-2M'_1} k_j + 2\sum_{j=1}^{M'_1} q_j \tag{9}$$

$$E = -2J \sum_{j}^{N-2M'_1} \cos(k_j) - 4J \sum_{j=1}^{M'_1} \cosh\xi_j \cos(q_j) + const. \tag{10}$$

where $q_j = \mathrm{Re}\,[k_{j1}] = \mathrm{Re}\,[k_{j2}]$ and $\xi_j = \mathrm{Im}\,[k_{j1}] = -\,\mathrm{Im}\,[k_{j2}]$, with $k_{j1}$ and $k_{j2}$ belonging to a length 2 $k - \Lambda$ string. Furthermore, it is possible to prove the following relation (see [2])

$$\cosh\xi_j = \sqrt{1 + \frac{U^2}{16J^2\cos^2(q_j)}}. \tag{11}$$

In the strongly interacting limit we have

$$-4J\cosh\xi_j\cos q_j \to U - 4J^2/|U| - 4J^2/|U|\cos(2q_j) + O\left(\frac{1}{U^2}\right) \tag{12}$$

which allows to write Eq. (10) as as

$$E = -2J \sum_{j}^{N-2M'_1} \cos(k_j) - 4J^2/|U| \sum_{j=1}^{M'_1} \cos(2q_j) + const. \tag{13}$$

The expression given by Eq. (13), corresponds to the dispersion of two different kind of particles, whose wavenumbers are respectively given by $k_j$ and $2q_j$. These objects are identified in the main text as doublons and unpaired particles.

From Eq. (10,11), it is possible to see that the initial BI state can be expressed as the $U \to \infty$ limit of the $N = 2M'_1$ eigenstate for the system. For finite $U$ the BI does not represent an eigenstate of the system, and therefore evolves following the dynamics generated by the Hubbard Hamiltonian, and which has been described in terms of two-site dynamics in the text.

## ANIMATION

In the animation we have depicted the time evolution of $log\,(n_u(t))$ for $U = 0$,$V_0 = 0$, $U = 0$, $V_0 = 5$; $U = 5$, $V_0 = 1$; $U = 10$, $V_0 = 0.5$. For all values of $UandV_0$, the most external wavefront propagates with velocity $2J$. In presence of interaction another front propagates with velocity $4J^2/U$. All three systems for which $V_0 \neq 0$ exhibit the same localization length (see also Fig. 3a. of the main text).

---

[1] F. M. Izrailev, S. Ruffo, and L. Tessieri, J Phys A-Math Gen **31**, 5263 (1999).
[2] F. H. L. Essler, et al., *The One-Dimensional Hubbard Model* (Cambridge University Press, 2005).
